# Supplementary material for: Bayesian Persuasion in Sequential Trials
Source: arXiv:2110.09594 source file (2021-11-22)
Supplement: Supplementary file 1 [file Z_Appendix.tex]

\section{Appendix: Discussions}

\subsection{Robustness of signaling strategies under small perturbation} \label{appendix:perturb}
Given the statement of Lemma~\ref{lem:nphasebp}, we are curious about the robustness of sender's optimal signaling strategy under small perturbations. Here, we want to discuss a 4-phase example which initially satisfies the conditions of Lemma \ref{lem:nphasebp} and see how small perturbations on trivial experiments will affect the sender's expected utility and the optimal signaling strategy.

To begin with, we consider a 4-phase example depicted in Figure \ref{fig:PerturbationGraph}, where $S^i$ denotes the $i^{th}$ sender-designed experiment, $N^i$ denotes the $i^{th}$ non-trivial experiment, and $T^i$ denotes the $i^{th}$ trivial experiment. The phase-I experiment is always $S^1$, then depends on the outcome of $S^1$, the phase-II experiment can be either $T^1$ or $N^1$ as depicted in the figure. To avoid ambiguity, for each experiment $E^i$, $q_1^{E^i},q_2^{E^i}$ represent the probability of going to the left node when the true state is $\theta_1,\theta_2$, respectively.
In this example, the prior belief of $\theta_1$ is set to be $p=0.4$, and all parameters of pre-determined experiments (trivial or non trivial) are provided in Table \ref{table:expparameter}.

\begin{figure}[ht]
    \centering
    \includegraphics[width=0.8\textwidth]{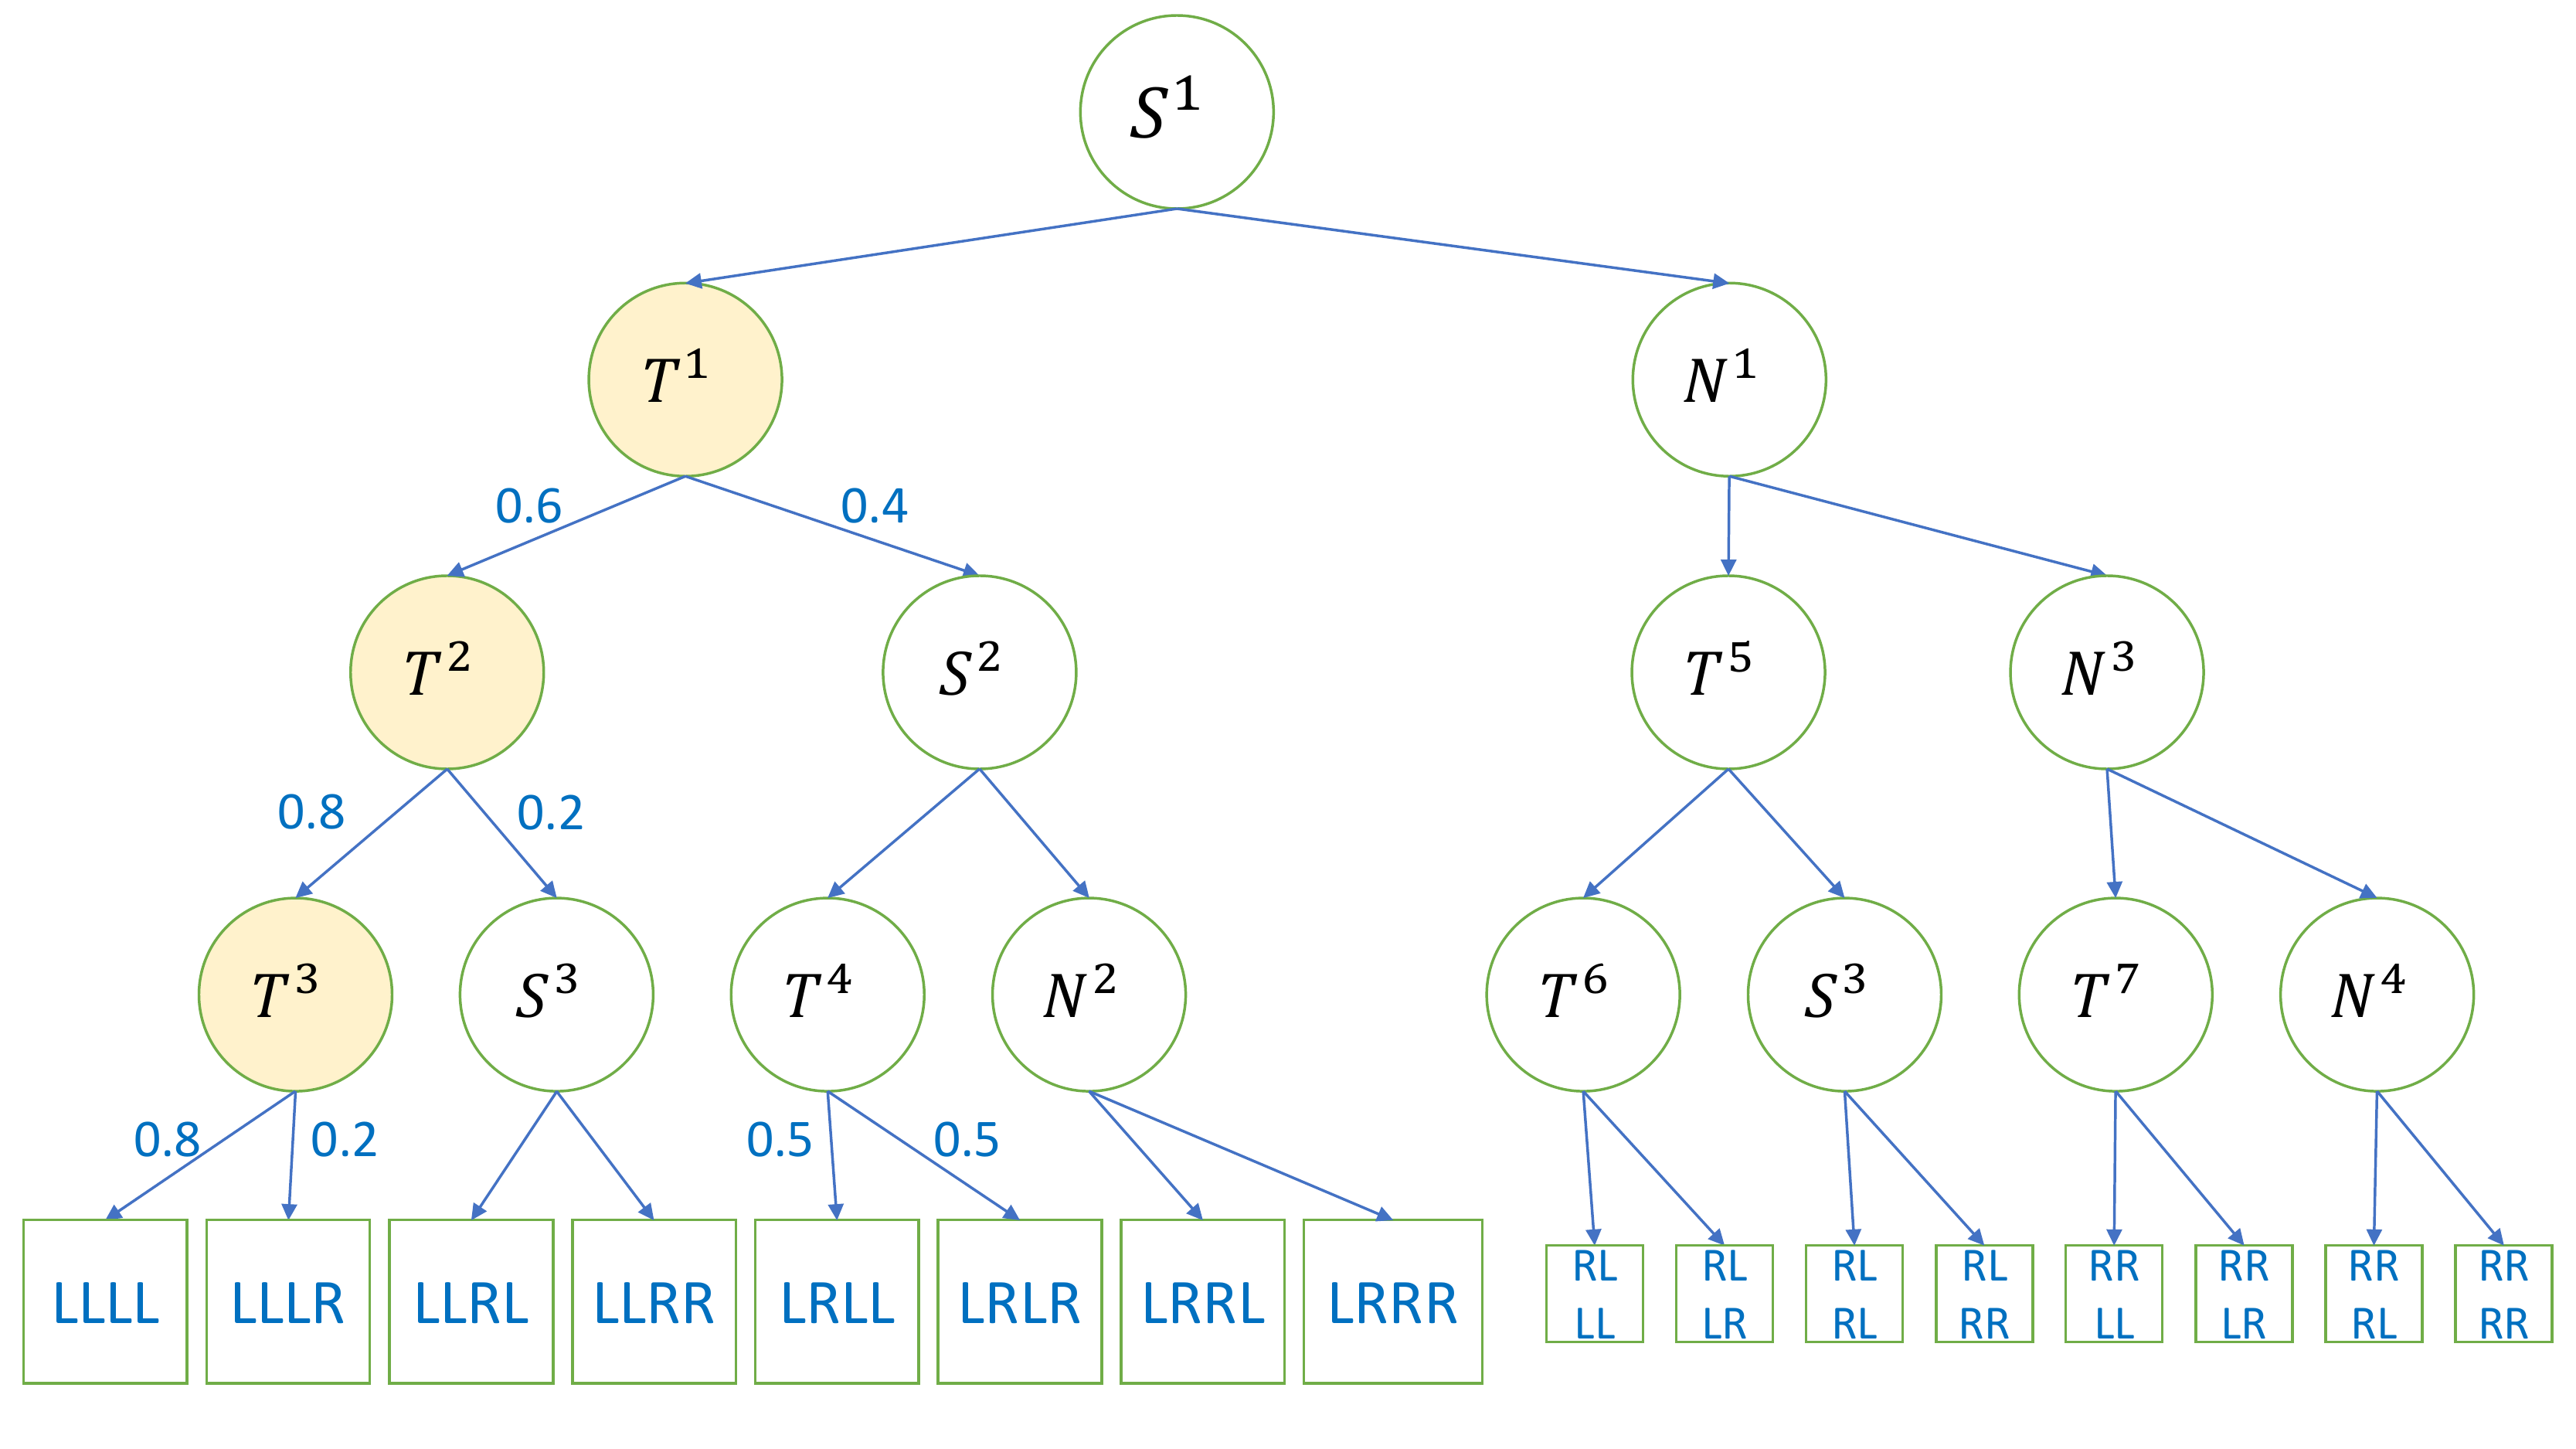}
    \caption{A four-phase trial satisfying Lemma~\ref{lem:nphasebp}}
    \label{fig:PerturbationGraph}
\end{figure}

\begin{table}[hb] 
\caption{Table of experiment parameters}
\centering
\label{table:expparameter}
\begin{tabular}{|c|c|c|c|c|c|c|c|c|c|c|c|} 
\hline
 Experiment& $T^1$ & $T^2$ &$T^3$&$T^4$&$T^5$&$T^6$&$T^7$&$N^1$&$N^2$&$N^3$&$N^4$ \\ \hline
 $q_1$& 0.6 & 0.8 &0.8 &0.5 &0.7 &0.7 &0.7 &0.8&0.6&1&0.5\\ \hline
 $q_2$& 0.4 & 0.2 &0.2 &0.5 &0.7 &0.7&0.7&0.5&0.4&0.5&0.5\\ \hline
\end{tabular}
\end{table}

When there is no perturbation, the sender's optimal signaling strategy will design $S^1$ to be $(q_1^{S^1},q_2^{S^2})=(1,\frac{2}{3})$ and the sender's expected utility is $0.8$. Now, we want to investigate small perturbations in $T^2$ and $T^3$. Since every trivial experiment $T^i$ has $q_1^{T^i}=q_2^{T^i}$, we assume that the perturbation always occurs in $q_2^{T^i}$ to avoid redundancy.

\paragraph{Example 1: Perturbation in $T_3$}
When there is a small perturbation of $q_2^{T^3}$, the posterior of the outcome $LLLL$ and $LLLR$ will now be different. In the original signaling strategy, the sender will make $\mathbb{P}(\theta_1|LLLL)=0.5$ and $\mathbb{P}(\theta_1|LLLR)=0.5$ to persuade the receiver taking action $\phi_1$. Under the perturbation, one of the outcome will have posterior belief less than $0.5$ and the receiver's best response will switch to $\phi_2$. Thus, the sender will have to decide whether she will accommodate this perturbation and design a new experiment at the very beginning ($S^1$) or using the same signaling strategy and reluctantly accept the loss. This utility change towards the perturbation is plotted in Figure \ref{fig:PerbutationT3}. We want to note that other examples with perturbation in the phase phase or in a trivial experiment where none of its succeeding experiments is a sender-designed experiment will have the figures with the shape similar to this one.
% \begin{figure}[htb]
%     \centering
%     \begin{subfigure}[b]{0.475\textwidth}
%         \centering
%         \includegraphics[width=0.95\textwidth,height=1.5in]{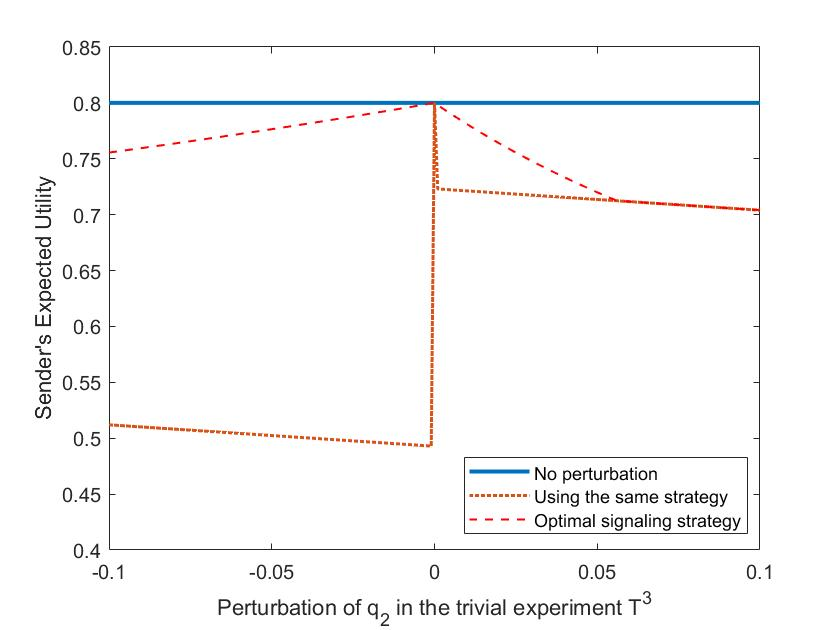}
%         \caption{Perturbation at $T^3$}
%         \label{fig:PerbutationT3}
%     \end{subfigure}
%     \hfill
%     \begin{subfigure}[b]{0.475\textwidth}
%         \centering
%         \includegraphics[width=0.95\textwidth,height=1.5in]{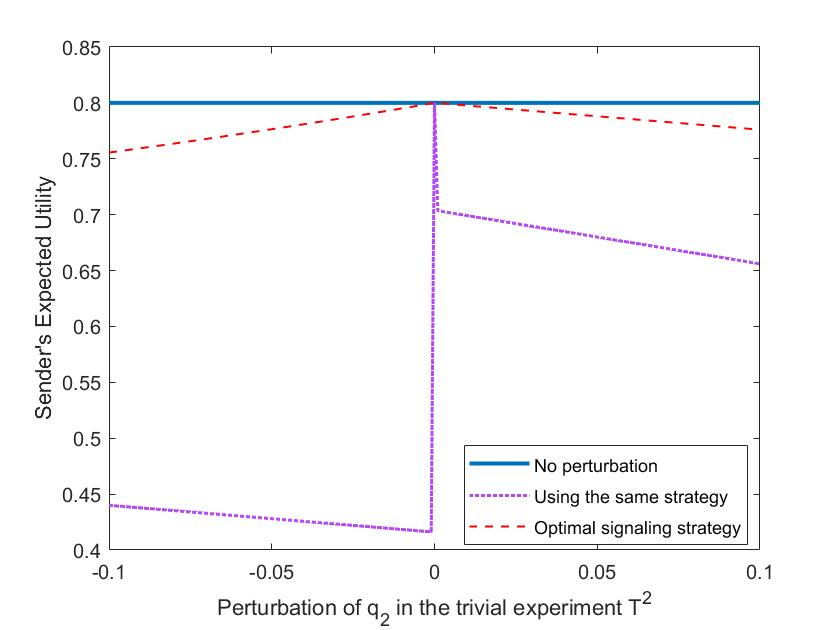}
%         \caption{Perturbation at $T^2$}
%         \label{fig:PerbutationT2}
%     \end{subfigure}
%     \caption{Robustness under perturbations to conditions of Lemma~\ref{lem:nphasebp}.}
%     \label{fig:my_label}
% \end{figure}
\begin{figure}[htb]
    \centering
        \includegraphics[scale=0.35]{perturbationT3.jpg}
    \caption{Perturbation at $T^3$}
    \label{fig:PerbutationT3}
\end{figure}

\paragraph{Example 2: Perturbation in $T_2$}
Instead of a perturbation in the last phase, we want to look at a perturbation occurs in a trivial experiment where one\footnote{If both of its succeeding experiments are sender-designed experiments, then the perturbation in this trivial experiment will not affect the sender's expected utility if it originally satisfies the conditions in Lemma \ref{lem:nphasebp}. The reason is the sender can design these two sender-designed experiments and adjust the sender-designed experiment in an earlier phase than this perturbation to cancel out the effect of a small perturbation.} of its succeeding experiment is a sender-designed experiment. In Figure \ref{fig:PerbutationT2}, different from Figure \ref{fig:PerbutationT3}, keeping the same strategy will never be an optimal when the perturbation increases the total probability on the side where its succeeding node is a sender-designed experiment. The reason is that when there is a sender-designed experiment in its succeeding, the sender can decide whether to accommodate the perturbation in earlier phases $S^1$ or in later phases $S^3$.

\begin{figure}[htb]
    \centering
    \includegraphics[scale=0.35]{perturbationT2.jpg}
    \caption{Perturbation at $T^2$}
    \label{fig:PerbutationT2}
\end{figure}

With above two small examples, we can see there's a significant utility drop even with a small perturbation. This suggests that even the difference between $q_{1}^E$ and $q_{2}^E$ is small, we should still view it as a non-trivial experiment instead of treating it as a trivial experiment.

\subsection{Solving Non-binary Experiments Directly}
Here, we want to present another dynamic programming operations to solve non-binary experiments directly. Again, supposing that we can solve the last two phases in non-binary outcome experiments directly via the LP, then the earlier phases can be solved by a dynamic programming approach similar to Section \ref{sec:multiphase}. 

To detail the dynamic programming operation in each experiment not in the last two phases, we again treat determined experiments and sender-designed experiments differently. Let's start with a determined experiment. Given a determined experiment in phase-$K$ with $n$ possible outcomes, denoted as $E_{K,i}=(q_{Ki11},,...,q_{Kin1},q_{Ki12},...q_{Kin2})$, if we have already solved the optimal persuasion ratio curves of its succeeding phase-$(K+1)$ experiments $E^i_{K+1,1}$, $E^i_{K+1,2}$, ..., $E^i_{K+1,n}$, represented by $PR^*_{K+1,(i,1)}(p)$, $PR^*_{K+1,(i,2)}(p)$, ..., $PR^*_{K+1,(i,n)}(p)$, then the optimal persuasion ratio curve at this determined phase-$K$ experiment $E_{K,i}$ is a linear combination of $PR^*_{K+1,(i,1)}(p)$, $PR^*_{K+1,(i,2)}(p)$, ..., $PR^*_{K+1,(i,n)}(p)$. It can be written in the following form:
\begin{eqnarray} 
    PR^*_{K,i}(p)=\sum_{j=1}^{n}(pq_{Kij1}+(1-p)q_{Kij2})PR^*_{K+1,(i,j)}\Big(\frac{pq_{Kij1}}{pq_{Kij1}+(1-p)q_{Kij2}}\Big).\label{eqn:3}
\end{eqnarray}

When we have an $n$-outcome experiment $E_{K,m}$ at phase K that the sender can design, the sender's optimal persuasion ratio curve is the generalized concave hull of all of its succeeding phase-$(K+1)$ experiments' persuasion ratio curves $PR^*_{K+1,(m,1)}(p)$, $PR^*_{K+1,(m,2)}(p)$, ..., $PR^*_{K+1,(m,n)}(p)$. This convex optimization function can be written in the following form:
\begin{eqnarray}
    PR^*_{K,m}(p)&=\displaystyle\max_{u_1,...u_n,~v_1,...v_n}\sum_{j=1}^{n}u_kPR^*_{K+1,(m,j)}\big(v_j\big) \label{eqn:4}\\
    \text{subject to}&
    \displaystyle\sum_{j=1}^{n}u_j=1,~\displaystyle\sum_{j=1}^{n}u_jv_j=p \nonumber
\end{eqnarray}

Given the convex optimization problem in (\ref{eqn:4}), we know that for each sender-designed experiment, we have to solve a convex optimization problem that has $2n-2$ parameters. At this point, we do not know whether it necessary to solve this optimization in its current form or whether some simplifications can be obtained that will drastically simplify this step. Answering this question is also for future work.

\subsection{Searching the optimal experiments from two sets with Lemma \ref{lem:inferior}} \label{appendix:usagelem7}
Consider a given experiment $E_A=(0.7,0.5)$. The receiver now can choose an experiment $E_B$ from two different sets. The first set has low $q_{B1}$ and low $q_{B2}$. It has to satisfying the following requirements:
\begin{enumerate}
    \item The experiment has a bounded pass rate, $0.1<q_{B2}\leq q_{B1}\leq 0.7$.
    \item The experiment has a limit of informativeness $q_{B1}-q_{B2}\leq 0.25$ and $\frac{q_{B1}}{q_{B2}}\leq1.6$.
\end{enumerate}
The second set has high pass rate $q_{B1},q_{B2}$ but it $q_{B1},q_{B2}$ are functions satisfying the following requirements:
\begin{enumerate}
    \item The experiment has a bounded pass rate, $0.7\leq q_{B1}\leq0.9$.
    \item $q_{B2}$ is a function of $q_{B1}$, $q_{B2}=1.05-2.5(1-q_{B1})$.
\end{enumerate}
The receiver wants to choose the experiment from one of these two sets to maximize her expected utility. 

Given Lemma~\ref{lem:inferior}, every other experiment in the first set is inferior to the experiment $(\frac{2}{3},\frac{5}{12})$. (Every experiment in the first set satisfying $q_{B1}\leq \frac{2-q_{B2}}{3-q_{B2}}$, hence, applying the first condition of Lemma \ref{lem:inferior} can help us build the partial order of experiments in the first set.) Hence, if the receiver will pick $E_B$ from the first set, she should choose the experiment $(\frac{2}{3},\frac{5}{12})$. 

In the second set, every experiment satisfies $q_{B1}> \frac{2-q_{B2}}{3-q_{B2}}$. Hence, we can use the second condition of Lemma \ref{lem:inferior} to build the partial order of this set of experiments. In this set, every other experiment is inferior to the experiment $(0.9,0.8)$. Thus, the receiver only needs to consider the experiment $(0.9,0.8)$.

Now, we check if we can order $(\frac{2}{3},\frac{5}{12})$ and $(0.9,0.8)$ directly using the inferiority defined in Definition \ref{dfn:inferior}. None of each is inferior to the other. Hence, we needs to look at whether the pair of experiments $\{(0.7,0.5), (\frac{2}{3},\frac{5}{12})\}$ gives the sender a higher expected utility than the pair $\{(0.7,0.5), (0.9,0.8)\}$. Explicit calculations show that the pair $\{(0.7,0.5), (\frac{2}{3},\frac{5}{12})\}$ gives the sender higher (or equal) expected utility for every prior. Hence, we can claim the receiver's optimal experiment in this example is $(\frac{2}{3},\frac{5}{12})$.

\subsection{Additional Real-world problems with multiple phases} \label{sec:extraexample}
In the introduction, we present a motivating interview example. Here, we want to provide more real-world Bayesian persuasion problems that contain multi-phase trials.

\subsubsection{Graduate application}
A junior undergraduate who wants to apply for graduate schools must submit her transcript and three recommendation letters from her professors. She wants to get offers no matter whether she is mature enough or not. The admission committee, who always wants to recruit mature students, will first do a GPA screening and then read the recommendation letters. The student can choose to take any combination of courses as she wishes, but the recommendation letters must come from the professors of taken courses. There are some easy courses with a high average GPA, but those instructors' recommendation letters tell minimal information of whether she is mature enough. 
On the contrary, there are lab courses that the instructor can tell whether she is mature enough but have a low average GPA. Now, the student has to decide the best combination of courses that she will take.

\subsubsection{Multi-round interview}
A new graduate wants to get an offer from a company. The department head of the company wants to hire a person who is competent for the position. To get an offer, the new graduate has to pass the interview. The interview has multiple rounds, and she can choose different strategies in each round to sell herself. According to her strength and personality traits that she shows in previous rounds, the department head will ask different questions in the final interview to evaluate whether the new graduate is competent for the position and decide whether the offer should be granted to the new graduate.

\subsubsection{Product Launch}
A product development team invents a new product and wants to launch it. The company has to decide whether it should launch such a new product or not. The product development team can decide the number of simplified trial products that will be sent out. Based on those trial products' customer feedback, the company will decide to offer it in different selected branches. Given the feedback and the sales report of branches, the company will decide whether to launch the product or not. 
\subsubsection{Advertisement of New products}
A company wants to sell a new product to a targeted customer, e.g., a cleaning robot, and the customer wants to buy the product if it is worth the money. The company can choose different advertisement methods to reach out to the customer, e.g., mailed ads, in-store posters, online ads, etc. After seeing the ads, the customer may choose different ways to evaluate whether it is worth buying the new product, conditional on how he saw the ads. Hence, a company must take the customer's possible evaluation technique into account while determining the best way to reach out to the customer.

\subsubsection{Buy-out}
A start-up wants to be acquired by a tech giant. The tech giant always wants to decide whether the acquisition will benefit its growth. To showcase its business model's potential, the start-up can first choose a consulting firm to evaluate some of its businesses. Based on the consulting firm's evaluation report, an accounting firm will audit these businesses' value, and the tech giant will decide based on both reports.

%\gs{this example is similar to the interview.}
% \subsubsection{Netflix Film}
% A production company wants people to watch their new film on Netflix. The company can choose a one-paragraph description, the tags it should add to the film, and a 60 seconds preview to attract couch potatoes. People search films using tags and pick one of the films matching these tags.
% {\color{red}This example is not good}

\subsection{Trade-off between efficiency and productivity}
In Bayesian persuasion problems, the signal strength (posterior beliefs of states under signals) and the signal distribution represent two different notions. The signal strength of a signal represents how efficiently\footnote{A signal $\omega$ is more efficient than $\omega'$ if the following statement is true: when we use the same total probability of the receiver' preferred state, which corresponds to the sender's suggested action of the signal ($\theta_1$ in this work), to implement both signals, the receiver's total probability of taking suggested action ($\phi_1$) while receiving $\omega$ is higher than the receiver's total probability of taking suggested action while receiving $\omega'$.} this signal can persuade the receiver. The signal distribution represents how productivity a signal strategy can benefit the sender under the current prior. However, in many (single-trial) Bayesian persuasion problems, e.g., binary-state space Bayesian persuasion, Bayesian persuasion with lexicographic-ordering senders\footnote{The sender has a lexicographic preference on actions.}, it is hard to evaluate the role that each notion plays in the optimal signaling strategy respectively. The reason is the insufficient degree of freedom on experiment design. To be more detailed, in those frameworks, the sender can always use the (set of) most efficient signals in the optimal signaling strategies. Given the (set of) most efficient signals, the most productive distribution can be solved by a greedy approach\footnote{Given the sender's preference on actions, the sender has a preference on signals (in terms of the efficiency). In this set of Bayesian persuasion problems, the sender can greedily pick the most efficient signal where the prior allows iteratively to come up the optimal signaling strategy.}. However, if we consider multi-phase trials, the trade-off between efficiency and productivity becomes the sender's primary issue (even in the binary-state space Bayesian persuasion problem with a lexicographic-ordering sender) because of the enlarged signal space. That is to say, if we want to get a better understanding of how the signal strength and the signal distribution plays a role in Bayesian persuasions respectively, it is not necessary to build complex models with stylized utility functions or increased state space. In this part, we demonstrate an example where the most efficient signal is not used in the sender's optimal signaling strategy owing to the trade-off between efficiency and productivity.

\vspace{4pt}
\hspace{-10pt}\textbf{Example:}

Given two pre-determined phase-II experiments $A,B$ with $(q_{A1},q_{A2})=(0.8,0.5)$ and $(q_{B1},q_{B2})=(0.75,0.15)$, we can derive the persuasion potential of $E_A$ and $E_B$, where $E_A=(1.6, 1.4)$ and $E_B=(1.5,\tfrac{9}{7})$. Under this persuasion potential, the most efficient signal will be a signal $\bar{\omega}$ with $(\mathbb{P}(\theta_1|\bar{\omega},E_A),\mathbb{P}(\theta_2|\bar{\omega}, E_A))=(\frac{5}{13},\frac{8}{13})$. As we can see, when the sender uses this signal, the sender is using the partial strategy $\alpha_A$ in her signaling strategy, and the IC constraint for $\alpha_A$ is tight. Here, we provide an example where the signal $\bar{\omega}$ is not in the support of the sender's optimal signaling strategy.

When the prior belief on state $\theta_1$, $p$, is $\frac{2}{3}$, we can solve the optimal signaling strategy for the sender using the approach developed in Section \ref{sec:BOE}. The optimal signaling strategy when $p=\frac{2}{3}$ is $(\beta_A,\alpha_B)$ with $\mathbb{P}(E_A,\theta_1)=\frac{55}{84}$ and $\mathbb{P}(E_A,\theta_2)=\frac{22}{84}$. The persuasion ratio of this optimal signaling strategy is $\frac{471}{336}	\approx 1.402$ and the sender's expected utility is $\frac{157}{168}\approx 0.935$. As we can see, the most efficient signal $\bar{\omega}$ is not in the support of the optimal signaling strategy. 

However, if the sender insists to use the signal $\bar{\omega}$, her best signaling strategy when $p=\frac{2}{3}$ is $(\alpha_A,\beta_B)$ with $\mathbb{P}(E_A,\theta_1)=\frac{5}{46}$ and $\mathbb{P}(E_A,\theta_2)=\frac{8}{46}$. The corresponding persuasion ratio is $\frac{123}{92}	\approx 1.337$ and the sender's expected utility is $\frac{41}{46}\approx 0.891$, which is lower than $\frac{157}{168}$ under the optimal signaling strategy. \hfill (The example is complete here)

\vspace{6pt}
In the above example, we demonstrate a case where using the most efficient signal is non-optimal in a two-phase trial's Bayesian persuasion problem. This example suggests that the sender has to consider the trade-off between efficiency and productivity to derive the optimal signaling strategy in multi-phase trials, which may not be necessary for single-trial Bayesian persuasion problems.
